# Supplementary material for: Inferring Interaction Rules From Observations of Evolutive Systems I: The Variational Approach
Source: arXiv:1602.00342 source file (2016-02-16)
Supplement: Supplementary file 1 [file appendix.tex]

% !TEX root = dynamicslearning.tex

\section{Appendix}

\subsection{Technical lemmas for the mean-field limit}\label{ap1}

The following preliminary result tells us that solutions to system \eqref{eq:discrdyn} are also solutions to systems \eqref{eq:contdyn}, whenever conveniently rewritten.

\begin{proposition}\label{p-rewritten}
Let $N \in \N$ be given. Let $(x^N_1, \ldots, x^N_N):[0,T] \rightarrow \R^{dN}$ be the solution of \eqref{eq:discrdyn} with initial datum $x^{N}_0 \in \R^{dN}$. Then the empirical measure $\mu^N:[0,T] \rightarrow \PP(\R^d)$ defined as in \eqref{eq:empmeas} is a solution of \eqref{eq:contdyn} with initial datum $\mu_{0}= \mu^N(0) \in \PC(\R^d)$.
\end{proposition}
\begin{proof}
It can be easily proved by arguing exactly as in \cite[Lemma 4.3]{MFOC}.
\end{proof}

 We are able to state several basic estimates that shall be useful towards an existence and uniqueness result for the solutions of system \eqref{eq:discrdyn}.

\begin{lemma}\label{p-estkernel}
Let $a\in X$ and $\mu \in \PP(\R^d)$. Then for all $y \in \R^d$ the following hold:
\begin{align*}
|(F[a] * \mu)(y)| \leq \|a\|_{L_{\infty}(\R_+)}\left( | y | + \int_{\R^d} | x | d\mu(x) \right).
\end{align*}
\end{lemma}
\begin{proof}
Trivially follows from $a \in L_{\infty}(\R_+)$.
\end{proof}

\begin{lemma}\label{p-Floclip}
If $a\in X$ then $F[a] \in \Lip_\loc(\R^d)$.
\end{lemma}
\begin{proof}
For any compact set $K \subset \R^d$ and for every $x,y \in K$ it holds
\begin{align*}
|F[a](x) - F[a](y)| &= |a(|x|)x - a(|y|)y| \\
&\leq |a(|x|)| |x-y| + |a(|x|) - a(|y|)| |y| \\
&\leq (|a(|x|)| + \Lip_K(a) |y|) |x-y|,
\end{align*}
and since $a \in L_{\infty}(\R_+)$ and $y \in K$, it follows that $F[a]$ is locally Lipschitz with Lipschitz constant depending only on $a$ and $K$.
\end{proof}

\begin{lemma}\label{p-Fmuloclip}
If $a\in X$ and $\mu \in \mathcal{P}_c(\R^d)$ then $F[a]*\mu \in \Lip_{\loc}(\R^d)$.
\end{lemma}
\begin{proof}
For any compact set $K \subset \R^d$ and for every $x,y \in K$ it holds
\begin{align*}
|(F[a]*\mu)(x) - (F[a]*\mu)(y)| &= \left|\int_{\R^d}a(|x-z|)(x-z)d\mu(z) - \int_{\R^d}a(|y-z|)(y-z)d\mu(z)\right| \\
&\leq \int_{\R^d}|a(|x-z|)-a(|y-z|)|x-z|d\mu(z)\\
&\quad+ \int_{\R^d}a(|y-z|)|x-y|d\mu(z) \\
&\leq \Lip_{\widehat{K}}(a)|x-y| \int_{\R^d}|x-z|d\mu(z) + \|a\|_{L_{\infty}(\R_+)}|x-y| \\
&\leq \left(\Lip_{\widehat{K}}(a)(|x| + 1)+ \|a\|_{L_{\infty}(\R_+)}\right)|x-y| \\
& \leq \left(C\Lip_{\widehat{K}}(a) + \|a\|_{L_{\infty}(\R_+)} \right)|x-y|,
\end{align*}
where $C$ is a constant depending on $K$, and $\widehat{K}$ is a compact set containing both $K$ and $\supp(\mu)$.
\end{proof}

\begin{proposition}
If $a \in X$ then system \eqref{eq:discrdyn} admits a unique global solution in $[0,T]$ for every initial datum $x^{N}_0 \in \R^{dN}$.
\end{proposition}
\begin{proof}
Rewriting system \eqref{eq:discrdyn} in the form of \eqref{eq:discr1}, from Lemma \ref{p-Fmuloclip} follows trivially that the function $G:\R^{dN} \rightarrow \R^{dN}$ defined for every $(x_1, \ldots, x_N)\in \R^{dN}$ as
\begin{align*}
G(x_1, \ldots, x_N) = ((F[a]*\mu^N)(x_1),\ldots,(F[a]*\mu^N)(x_N)),
\end{align*}
where $\mu^N$ is the empirical measure given by \eqref{eq:empmeas}, satisfies $G \in \Lip_\loc(\R^{dN})$. The Cauchy-Lipschitz Theorem for ODE systems then yields the desired result.
\end{proof}

Variants of the following result are \cite[Lemma 6.7]{MFOC} and \cite[Lemma 4.7]{CanCarRos10}

\begin{lemma}\label{p-lipkernel}
Let $a \in X$ and let $\mu:[0,T] \rightarrow \mathcal{P}_c(\R^d)$ and $\nu: [0,T] \to \PP(\R^d)$ be two continuous maps with respect to $\W_1$ satisfying
\begin{align}\label{eq:bsupp}
\supp(\mu(t)) \cup \supp(\nu(t)) \subseteq B(0,R),
\end{align}
for every $t \in [0,T]$, for some $R > 0$. Then for every $r > 0$ there exists a constant $L_{a,r,R}$ such that
\begin{align}\label{eq:inftynormW1}
\|F[a] * \mu(t) - F[a] * \nu(t)\|_{L_{\infty}(B(0,r))} \leq L_{a,r,R} \W_1(\mu(t),\nu(t))
\end{align}
for every $t \in [0,T]$.
\end{lemma}
\begin{proof}
Fix $t \in [0,T]$ and take $\pi \in \Gamma_o(\mu(t),\nu(t))$. Since the marginals of $\pi$ are by definition $\mu(t)$ and $\nu(t)$, it follows
\begin{align*}
F[a] * \mu(t)(x) - F[a] * \nu(t)(x) &= \int_{B(0,R)} F[a](x-y) d\mu(t)(y) - \int_{B(0,R)} F[a](x-z) d\nu(t)(z)  \\
&= \int_{B(0,R)^2} \left(F[a](x-y) - F[a](x-z)\right) d\pi(y,z)
\end{align*}
By using Lemma \ref{p-Floclip} and the hypothesis \eqref{eq:bsupp}, we have
\begin{align*}
\|F[a] * \mu(t) - F[a] * \nu(t)\|_{L_{\infty}(B(0,r))} &\leq \esssup_{x \in B(0,r)} \int_{B(0,R)^2} \left|F[a](x-y) - F[a](x-z)\right| d\pi(y,z) \\
&\leq \Lip_{B(0,R+r)}(F[a]) \int_{B(0,R)^2} |y - z| d\pi(y,z) \\
&= \Lip_{B(0,R+r)}(F[a]) \W_1(\mu(t),\nu(t)),
\end{align*}
hence \eqref{eq:inftynormW1} holds with $L_{a,r,R} = \Lip_{B(0,R+r)}(F[a])$.
\end{proof}

\subsection{Proof of Proposition \ref{pr:exist}}\label{ap2}

Notice that for every $N \in \N$, by Proposition \ref{p-rewritten}, $\mu^N$ is the unique solution of \eqref{eq:contdyn} with initial datum $\mu^N_0$. We start by fixing $N \in \N$ and estimating the growth of $|x_i^N(t)|^2$ for $i = 1, \ldots, N$. By using Lemma \ref{p-estkernel}, we have
\begin{align*}
\frac{1}{2}\frac{d}{dt} |x_i^N(t)|^2 & \leq \dot{x}_i^N(t) \cdot x_i^N(t) \\
& \leq \left|(F[a]*\mu^N(t))(x_i(t))\right| |x_i^N(t)| \\
& \leq \|a\|_{L_{\infty}(\R_+)}\left( |x_i^N(t)| + \frac{1}{N} \sum^N_{j = 1}|x_j^N(t)| \right) |x_i^N(t)| \\
& \leq 2 \|a\|_{L_{\infty}(\R_+)}\max_{j = 1, \ldots, N} |x_j^N(t)| |x_i^N(t)| \\
& \leq 2 \|a\|_{L_{\infty}(\R_+)}\max_{j = 1, \ldots, N} |x_j^N(t)|^2.
\end{align*}
If we denote by $q(t) := \max_{j = 1, \ldots, N} |x_j^N(t)|^2$, then the Lipschitz continuity of $q$ implies that $q$ is a.e. differentiable. Stampacchia's Lemma \cite[Chapter 2, Lemma A.4]{Kin-Sta} ensures that for a.e. $t \in [0,T]$ there exists $k = 1, \ldots, N$ such that
\begin{align*}
\dot{q}(t) = \frac{d}{dt} |x_k^N(t)|^2 \leq 4 \|a\|_{L_{\infty}(\R_+)} q(t).
\end{align*}
Hence, Gronwall's Lemma and the hypothesis $x^{N}_{0,i} \in \supp(\mu_0) + \overline{B(0,1)}$ for every $N \in \N$ and $i = 1, \ldots, N$, imply that
\begin{align*}
q(t) \leq q(0) e^{4 \|a\|_{L_{\infty}(\R_+)} t} \leq C_0 e^{4 \|a\|_{L_{\infty}(\R_+)} t} \text{ for a.e. } t \in [0,T],
\end{align*}
for some uniform constant $C_0$ depending only on $\mu_0$. Therefore, the trajectory $\mu^N(\cdot)$ is bounded uniformly in $N$ in a ball $B(0,R) \subset \R^d$, where
\begin{align}\label{Rest}
R =  \sqrt{C_0} e^{2 \|a\|_{L_{\infty}(\R_+)} T}.
\end{align}
This, in turn, implies that $\mu^N(\cdot)$ is Lipschitz continuous with Lipschitz constant uniform in $N$, since by the fact that $|x^N_i(t)| \leq R$ for a.e. $t \in [0,T]$, for all $N \in N$ and $i = 1, \ldots, N$, and Lemma \ref{p-estkernel} follows
\begin{align*}
|\dot{x}^N_i(t)| &= |(F[a]*\mu^N(t))(x^N_i(t))| \\
&\leq \|a\|_{L_{\infty}(\R_+)} \left( |x^N_i(t)| + \frac{1}{N}\sum^N_{j = 1}|x^N_j(t)|\right) \\
&\leq 2R\|a\|_{L_{\infty}(\R_+)}.
\end{align*}
We have thus found a sequence $(\mu^N)_{N \in \N} \subset \mathcal{C}^0([0,T],\mathcal{P}_1(B(0,R)))$ for which the following holds:
\begin{itemize}
\item $(\mu^N)_{N \in \N}$ is equicontinuous and closed, because of the uniform Lipschitz constant $2R\|a\|_{L_{\infty}(\R_+)}$;
\item for every $t \in [0,T]$, the sequence $(\mu^N(t))_{N \in \N}$ is relatively compact in $\mathcal{P}_1(B(0,R))$. This holds because $(\mu^N(t))_{N \in \N}$ is a tight sequence, since $B(0,R)$ is compact, and hence relatively compact due to Prokhorov's Theorem.
\end{itemize}
Therefore, we can apply the Ascoli-Arzel\'{a} Theorem for functions with values in a metric space (see for instance, \cite[Chapter 7, Theorem 18]{KelleyTop}) to infer the existence of a subsequence $(\mu^{N_k})_{k \in \N}$ of $(\mu^N)_{N \in \N}$ such that
\begin{align}\label{eq:unifconv}
\lim_{k \rightarrow \infty}\W_1(\mu^{N_k}(t),\mu(t)) = 0 \quad \text{ uniformly for a.e. } t \in [0,T],
\end{align}
for some $\mu \in \mathcal{C}^0([0,T],\mathcal{P}_1(B(0,R)))$ with Lipschitz constant bounded by $2R\|a\|_{L_{\infty}(\R_+)}$. The hypothesis $\lim_{N\rightarrow\infty}\W_1(\mu^N_0,\mu_0) = 0$ now obviously implies $\mu(0) = \mu_0$.

We are now left with verifying that this curve $\mu$ is a solution of \eqref{eq:contdyn}. For all $t \in [0,T]$ and for all $\varphi \in \mathcal{C}^1_c(\R^d;\R)$, since it holds
\begin{align*}
\frac{d}{dt}\langle \varphi, \mu^N(t) \rangle = \frac{1}{N}\frac{d}{dt} \sum^N_{i = 1} \varphi(x^N_i(t)) = \frac{1}{N} \sum^N_{i = 1} \nabla\varphi(x^N_i(t)) \cdot \dot{x}_i^N(t),
\end{align*}
by directly applying the substitution $\dot{x}_i^N(t) = (F[a]*\mu^N(t))(x^N_i(t))$, we have
\begin{align*}
\langle \varphi, \mu^N(t) - \mu^N(0) \rangle = \int^t_0 \left[ \int_{\R^d}\nabla \varphi(x) \cdot (F[a]*\mu^N(s))(x) d\mu^N(s)(x) \right] ds.
\end{align*}
By Lemma \ref{p-lipkernel}, the inequality \eqref{eq:unifconv}, and the compact support of $\varphi \in \mathcal{C}^1_c(\R^d;\R)$, follows
\begin{align*}
\lim_{N \rightarrow \infty} \|\nabla\varphi \cdot (F[a]*\mu^N(t) - F[a]*\mu(t))\|_{L_{\infty}(\R^d)} = 0 \quad \text{ uniformly for a.e. } t \in [0,T].
\end{align*}
If we denote with $\mathcal L_1\llcorner_{[0,t]}$ the Lebesgue measure on the time interval $[0,t]$, since the product measures $\frac{1}{t} \mu^{N}(s) \times \mathcal L_1\llcorner_{[0,t]}$ converge in $\mathcal P_1([0,t] \times \mathbb R^{d})$ to $\frac{1}{t} \mu(s) \times \mathcal L_1\llcorner_{[0,t]}$, we finally get from the dominated convergence theorem that
\begin{align*}
\lim_{N \to \infty} \int_0^{t} \int_{\mathbb R^{d}} \nabla \phi(x) \cdot (F[a]*&\mu^N(s))(x) d\mu^N(s)(x) ds \\
&=  \int_0^{t} \int_{\mathbb R^{d}} \nabla \phi(x) \cdot (F[a]*\mu(s))(x) d \mu(s)(x) ds,
\end{align*}
which proves that $\mu$ is a solution of \eqref{eq:contdyn} with initial datum $\mu_0$.

\subsection{Existence and uniqueness of solutions for  \eqref{eq:transpdyn}}\label{ap3}

For the reader's convenience we start by briefly recalling some general, well-known results about solutions to Carath{\'e}odory differential equations. We fix a domain $\Omega \subset \R^d$, a Carath{\'e}odory function $g\colon[0,T]\times \Omega \to \R^d$, and $0<\tau \le T$. A function $y\colon [0,\tau]\to \Omega$ is called a solution of the Carath{\'e}odory differential equation
\begin{equation}\label{cara}
\dot y(t)=g(t, y(t))
\end{equation}
on $[0,\tau]$ if and only if $y$ is absolutely continuous and \eqref{cara} is satisfied a.e.\ in $[0,\tau]$.
The following existence result holds.
%\begin{theorem}\label{cara2}
%Consider an interval $[0,T]$ on the real line and a domain $\Omega \subset \R^n$, for $n\ge 1$. Let $g\colon[0,T]\times \Omega \to \R^n$ be a Carath{\'e}odory function for which there exists a function $m \in L_1((0,T))$ such that
%$$
%|g(t,y)|\le m(t)
%$$
%for a.e.\ $t \in [0,T]$ and every $y \in \Omega$. Then, given $y_0 \in \Omega$, there exists $0<\tau \le T$ and a solution $y(t)$ of \eqref{cara} on $[0,\tau]$ satisfying $y(0)=y_0$. 
%
%If in addition there exists a function $l \in L_1((0,T))$ such that
%\begin{equation}\label{cara3}
%|g(t,y_1)-g(t, y_2)|\le l(t)|y_1-y_2|
%\end{equation}
%for a.e.\ $t \in [0,T]$ and every $y_1$, $y_2 \in \Omega$, the solution is uniquely determined on $[0,\tau]$ by the initial condition $y_0$.
%\end{theorem}
%
%\begin{proof}
%See, for instance, \cite[Chapter 1, Theorems 1 and 2]{Fil}.
%\end{proof}
%
%What follows is a generalization of the global existence theorem and of a Gronwall-type estimate on the solutions to this setting.

\begin{theorem}\label{cara-global}
Fix $T > 0$ and $y_0 \in \R^d$. Suppose that there exists a compact subset $\Omega$ of $\R^d$ such that $y_0 \in \textup{int}(\Omega)$ and there exists $m_{\Omega} \in L_1([0,T])$ for which it holds
%Consider an interval $[0,T]$ on the real line, a compact subset $K$ of $\R^n$, and a Carath{\'e}odory function $g\colon[0,T]\times \R^n \to \R^n$. If there exists a function $m \in L_1((0,T))$ such that
\begin{align}\label{l1}
|g(t,y)|\le m_{\Omega}(t),
\end{align}
for a.e.\ $t \in [0,T]$ and for all $y \in \Omega$. Then there exists a $\tau > 0$ and a solution $y(t)$ of \eqref{cara} defined on the interval $[0,\tau]$ which satisfies $y(0)=y_0$. If there exists $C > 0$ such that the function $g$ also satisfies the condition
\begin{align}\label{ttz}
|g(t,y)|\le C(1+|y|),
\end{align}
for a.e.\ $t \in [0,T]$ and every $y \in \Omega$, and it holds $B(0,R) \subseteq \Omega$, for $R > |y_0| + CT e^{CT}$, then the local solution $y(t)$ of \eqref{cara} which satisfies $y(0)=y_0$ can be extended to the whole interval $[0,T]$. Moreover, for every $t \in [0,T]$, any solution satisfies
\begin{equation}\label{gron}
|y(t)|\le \Big(|y_0|+ Ct\Big) \,e^{Ct}.
\end{equation}
%If in addition, for every relatively compact open subset $\Omega \subset \R^d$ there exists a constant $L_{\Omega}$ for which it holds
%\begin{align}\label{cara3}
%|g(t,y_1)-g(t, y_2)|\le L_{\Omega}|y_1-y_2|,
%\end{align}
%for a.e.\ $t \in [0,T]$ and every $y_1$, $y_2 \in \Omega$, then the solution is uniquely determined on $[0,T]$ by the initial condition $y_0$.
\end{theorem}

\begin{proof}
%Set $\rho:= (|y_0|+CT) \,e^{CT}$ and
Since $y_0 \in \textup{int}(\Omega)$, we can consider a ball $B(y_0,r) \subset \Omega$. The classical result \cite[Chapter 1, Theorem 1]{Fil} and \eqref{l1} yield the existence of a local solution defined on an interval $[0,\tau]$ and taking values in $B(y_0,r)$.

If \eqref{ttz} holds, any solution of \eqref{cara} with initial datum $y_0$ satisfies
$$
|y(t)|\le |y_0|+ Ct+C\int_0^t |y(s)|\,ds
$$
for every $t \in [0,\tau]$, therefore \eqref{gron} follows from Gronwall's inequality. In particular the graph of a solution $y(t)$ cannot reach the boundary of $[0,T]\times B(0,|y_0|+CTe^{CT})$ unless $\tau=T$, therefore the continuation of the local solution to a global one on $[0,T]$ follows, for instance, from \cite[Chapter 1, Theorem 4]{Fil}.
%Finally, if \eqref{cara3} holds, uniqueness of the global solution follows from \cite[Chapter 1, Theorem 2]{Fil}.
\end{proof}

Gronwall's inequality easily gives us the following results on continuous dependence on the initial data.

\begin{lemma}\label{le:uniquecara}
Let $g_1$ and $g_2\colon[0,T]\times \R^n \to \R^n$ be Carath{\'e}odory functions both satisfying \eqref{ttz} for the same  constant $C > 0$. Let $r>0$ and define 
\begin{align*}
\rho_{r, C, T}:=\Big(r+ CT\Big) \,e^{CT}\,.
\end{align*}
Assume in addition that there exists a constant $L > 0$ satisfying
\begin{align*}
|g_1(t, y_1)-g_1(t, y_2)|\le L|y_1-y_2|
\end{align*}
for every $t \in [0, T]$ and every $y_1$, $y_2$ such that $|y_i|\le \rho_{r, C, T}$, $i=1,2$.
Then, if $\dot y_1(t)=g_1(t, y_1(t))$, $\dot y_2(t)=g_2(t, y_2(t))$, $|y_1(0)|\le r$ and $|y_2(0)|\le r$, one has
\begin{equation}\label{gronvalla}
|y_1(t)-y_2(t)|\le e^{Lt}\left(|y_1(0)-y_2(0)|+\int_0^t \|g_1(s, \cdot)-g_2(s, \cdot)\|_{L_\infty(B(0, \rho_{r, C, T}))} \,ds \right)
\end{equation}
for every $t \in [0, T]$.
\end{lemma}
\begin{proof}
We can bound $|y_1(t) - y_2(t)|$ from above as follows:
\begin{align*}
|y_1(t) - y_2(t)| &\leq |y_1(0) - y_2(0)| + \int^t_0 |\dot{y}_1(s) - \dot{y}_2(s)| ds \\
&= |y_1(0) - y_2(0)| \\
& \quad + \int^t_0 |g_1(s, y_1(s)) - g_1(s, y_2(s)) + g_1(s, y_2(s)) - g_2(s, y_2(s))| ds \\
& \leq |y_1(0) - y_2(0)| + \int_0^t \|g_1(s, \cdot)-g_2(s, \cdot)\|_{L_\infty(B(0, \rho_{r, C, T}))} \,ds \\
& \quad  + L \int^t_0|y_1(s) - y_2(s)| ds.
\end{align*}
Since the function $\alpha(t) = |y_1(0) - y_2(0)| + \int_0^t \|g_1(s, \cdot)-g_2(s, \cdot)\|_{L_\infty(B(0, \rho_{r, C, T}))} \,ds$ is increasing, an application of Gronwall's inequality gives \eqref{gronvalla}, as desired.
\end{proof}

\begin{proposition}
Fix $T > 0$, $a \in X$, $\mu_0 \in \mathcal{P}_c(\R^d)$, $\xi_0 \in \R^d$ and let $R > 0$ be given by Proposition \ref{pr:exist} from the choice of $T, a$ and $\mu_0$. For every map $\mu:[0,T] \rightarrow \PP(\R^d)$ which is continuous with respect to $\W_1$ such that
\begin{align*}
\supp(\mu(t)) \subseteq B(0,R) \quad \text{ for every } t \in [0,T],
\end{align*}
there exists a unique solution of system \eqref{eq:transpdyn} with initial value $\mu_0$ defined on the whole interval $[0,T]$.
\end{proposition}
\begin{proof}
By Lemma \ref{p-estkernel} follows that, for any compact set $K \subset \R^d$ containing $\xi_0$, there exists a function $m_K \in L_1([0,T])$ for which the function $g(t,y)=(F[a]\ast\mu(t))(y)$ satisfies \eqref{l1}. Moreover, for fixed $t$ this function is locally Lipschitz continuous, as follows from Lemma \ref{p-Fmuloclip}, thus $g(t,y)=(F[a]\ast\mu(t))(y)$ is a Carath\'eodory function.

%Notice that $a \in L_{\infty}(\R_+)$ trivially implies that of $F[a] \in L_{\infty}_{\loc}(\R^d)$. This, together with Lemma \ref{p-estkernel} and the hypothesis that $\supp(\mu(t)) \subseteq B(0,R)$ for all $t \in [0,T]$, yields $F[a]\ast\mu(t)\in L_{\infty}(\R_+)$ uniformly in $t$, hence \eqref{l1} holds. 
		
From the hypothesis that the support of $\mu$ is contained in $B(0,R)$ and Lemma \ref{p-estkernel}, follows the existence of a constant $C$ depending on $T,a$ and $\mu_0$ such that
\begin{align*}
|(F[a]*\mu(t))(y)| &\leq C(1+|y|)
\end{align*}
holds for every $y \in \R^d$ and for every $t \in [0,T]$. Hence $F[a]*\mu(t)$ is sublinear and \eqref{ttz} holds. By considering a sufficiently large compact set $K$ containing $\xi_0$, Theorem \ref{cara-global} guarantees the existence of a solution of system \eqref{eq:transpdyn} defined on $[0,T]$.

To establish uniqueness notice that, from Lemma \ref{p-Floclip}, for every compact subset $K \in \R^d$ and any $x,y \in K$, it holds
\begin{align}
\begin{split}\label{eq:uniquecara}
|(F[a]*\mu(t))(x) - (F[a]*\mu(t))(y)| &\leq \left| \int_{\R^d}F[a](x-z)d\mu(t)(z) - \int_{\R^d}F[a](y-z)d\mu(t)(z)\right| \\
&\leq \int_{\R^d} \left|F[a](x-z) - F[a](y-z)\right|d\mu(t)(z) \\
&\leq \Lip_{\widehat{K}}(F[a]) |x-y|,
\end{split}\end{align}
where $\widehat{K}$ is a compact set containing both $K$ and $B(0,R)$. Hence, uniqueness follows from \eqref{eq:uniquecara} and Lemma \ref{le:uniquecara} by taking $g_1 = g_2$, $y_1(0) = y_2(0)$ and $r = |y_1(0)|$.
\end{proof}

\subsection{Continuous dependence on the initial data}\label{ap4}

The following Lemma and \eqref{gronvalla} are the main ingredients of the proof of Theorem \ref{uniq} on continuous dependance on initial data.

\begin{lemma}\label{primstim}
Let $\mathcal{T}_1$ and $\mathcal{T}_2 \colon \R^n \to \R^n$ be two bounded Borel measurable functions. Then, for every $\mu \in \PP(\R^n)$ one has
\begin{align*}
\W_1((\mathcal{T}_1)_{\#}\mu, (\mathcal{T}_2)_{\#} \mu) \le \|\mathcal{T}_1-\mathcal{T}_2\|_{L_\infty({\rm supp}\,\mu)}.
\end{align*}
If in addition $\mathcal{T}_1$ is locally Lipschitz continuous, and $\mu$, $\nu \in \PP(\R^n)$ are both compactly supported on a ball $B(0,r)$ of $\R^n$, then
\begin{align*}
\W_1((\mathcal{T}_1)_{\#} \mu, (\mathcal{T}_1)_{\#} \nu) \le \Lip_{B(0,r)}(E_1) \W_1(\mu, \nu).
\end{align*}
\end{lemma}

\begin{proof}
See \cite[Lemma 3.11]{CanCarRos10} and \cite[Lemma 3.13]{CanCarRos10}.
\end{proof}

We can now prove Theorem \ref{uniq}.

\begin{proof}[Proof of Theorem \ref{uniq}]
Let  ${\mathcal T}^\mu_t$ and ${\mathcal T}^\nu_t$ be the flow maps associated to system \eqref{eq:transpdyn} with measure $\mu$ and $\nu$, respectively.
By \eqref{eq:fixedpoint}, the triangle inequality, Lemma \ref{p-lipkernel}, Lemma \ref{primstim} and \eqref{eq:liptrans} we have for every $t \in [0,T]$
\begin{align}
\begin{split}\label{start}
\W_1(\mu(t), \nu(t))&=\W_1(({\mathcal T}^\mu_t)_{\#} \mu_0, ({\mathcal T}^\nu_t)_{\#} \nu_0)  \\
&\le \W_1(({\mathcal T}^\mu_t)_{\#} \mu_0, ({\mathcal T}^\mu_t)_{\#} \nu_0) + \W_1(({\mathcal T}^\mu_t)_{\#} \nu_0, ({\mathcal T}^\nu_t)_{\#} \nu_0)\\
&\le e^{T \, \Lip_{B(0,R)}(F[a])} \W_1(\mu_0, \nu_0)+\|{\mathcal T}^\mu_t-{\mathcal T}^\nu_t\|_{L_\infty(B(0,R))}.
\end{split}
\end{align}

Using \eqref{gronvalla} with $y_1(0)= y_2(0)$ we get
\begin{equation}\label{stima2}
\|{\mathcal T}^\mu_t-{\mathcal T}^\nu_t\|_{L_\infty(B(0,r))}\le e^{t \, \Lip_{B(0,R)}(F[a])}\int_0^t \|F[a]* \mu(s)-F[a]* \nu(s)\|_{L_\infty(B(0,R))}\,ds.
\end{equation}

Combining \eqref{start} and \eqref{stima2} with Lemma \ref{p-lipkernel}, we have
$$
\W_1(\mu(t), \nu(t))\le e^{T \, \Lip_{B(0,R)}(F[a])} \left(\W_1(\mu_0, \nu_0)+ L_{a,R,R}\int_0^t \W_1(\mu(s), \nu(s)) \,ds\right)
$$
for every $t \in [0, T]$, where $L_{a,R,R}$ is the constant from Lemma \ref{p-lipkernel}. Gronwall's inequality now gives
$$
\W_1(\mu(t), \nu(t))\le e^{T \, \Lip_{B(0,R)}(F[a]) + L_{a,R,R}} \W_1(\mu_0, \nu_0),
$$
which is exactly \eqref{stab} with $\overline{C}= e^{T \, \Lip_{B(0,R)}(F[a]) + L_{a,R,R}}$.

Consider now two solutions of \eqref{eq:contdyn} with the same initial datum $\mu_0$. Since, from Proposition \ref{pr:exist} they both satisfy \eqref{supptot} for the given \textit{a priori known} $R$ given by \eqref{Rest}, then \eqref{stab} guarantees they both describe the same curve in $\PP(\R^d)$. This concludes the proof.
\end{proof}
